# Supplementary material for: Systems-Theoretic Safety Assessment of Teleoperated Road Vehicles
Source: arXiv:2104.06795 source file (2021-04-14)
Supplement: Supplementary file 1 [file Appendix.tex]

\section*{\uppercase{Appendix}}
